# Supplementary material for: Quantization of charged fields in the presence of intense electromagnetic fields
Source: arXiv:2510.09447 source file (2025-10-10)
Supplement: Supplementary file 1 [file 06-Appendices.tex]

\ifthenelse{\equal{\LanguageOption}{portuguese}}{
    \addtocontents{toc}{\protect\contentsline{chapter}{Apêndices}{}{}}
}{
    \addtocontents{toc}{\protect\contentsline{chapter}{Appendices}{}{}}
}

\blankpage
\begin{center}
    %\minionfont
    \thispagestyle{empty}
        
    \vspace*{\fill}
    \ifthenelse{\equal{\LanguageOption}{portuguese}}{%
        {\LARGE\fontsize{26}{26}\selectfont\textcolor{darkred}{Apêndices}\par}
    }{%
        {\LARGE\fontsize{26}{26}\selectfont\textcolor{darkred}{Appendices}\par}
    }
    \vspace*{\fill}
\end{center}
\blankpage
